# Supplementary material for: Distributed Freeze Tag: a Sustainable Solution to Discover and Wake-up a Robot Swarm
Source: arXiv:2503.22521 source file (2025-03-28)
Supplement: Supplementary file 1 [file old-appendix.tex]

\section{Unit Disk Graph}
\subsection{High-level description of the algorithm}
We present a synchronized algorithm that aims to mimic a breadth first search in the underlying UDG: at each round, (1) each awake robot $u$ select a part of its sleeping neighbourhood up using a simple selection process, (2) computes a wake up tree and (3) propagates the awakening process in its ball $B_u$.

\paragraph{Selection process:}

If $u$ and $v$ have been awakened in the previous round and $B_u \cap B_v$ contains a sleeping robot $w$, it is simple to decide locally the robot that will have in charge $w$ whenever $|uv| \leq 1$. This can be done using \emph{the closest selection rule}. The main difficulty is to handle conflicts if $|uv| > 1$. The main trick is to partition each ball into $6$ sectors of similar angles and to compute wake up trees in parallel for the corresponding sector.  For any robot $u$, $B_u$ is divided into $6$ circular sector and $u$ wakes up sectors one by one, breaking down the wake up of $B_u$ into a round of $6$ phases of fixed duration. We show with Lemma~\ref{lem:conflit} that this staggering allows synchronization between robots that may interfere with each other.

\paragraph{Wake up tree computation in $B_u$.}

Once a robot $u$ knows the set of sleeping robots to handle within a sector, $u$ can wake up its unit ball $B_u$ in constant time using a centralized algorithm. 

\subsubsection{Selection process}

A \emph{sector} of a unit ball $B_u$ is the intersection of $B_u$ and the region in the plane between two rays that emanate from $u$, its apex. If the position of $u$ is $p$, for $i \in [1,6]$, $a_i$ is the intersection the unit circle centered at $p$ and the ray of apex $p$ and of angle $\frac{(i-1) \pi}{3}$. We denote by $B_u^i$ the $i$-th  sector of $B_u$ defined by an arc from $a_i$ to $a_{i+1}$ (cf. fig. \ref{fig:def-sector}).

\begin{figure}[htbp!]
    \centering
    \includegraphics[width=0.5\linewidth]{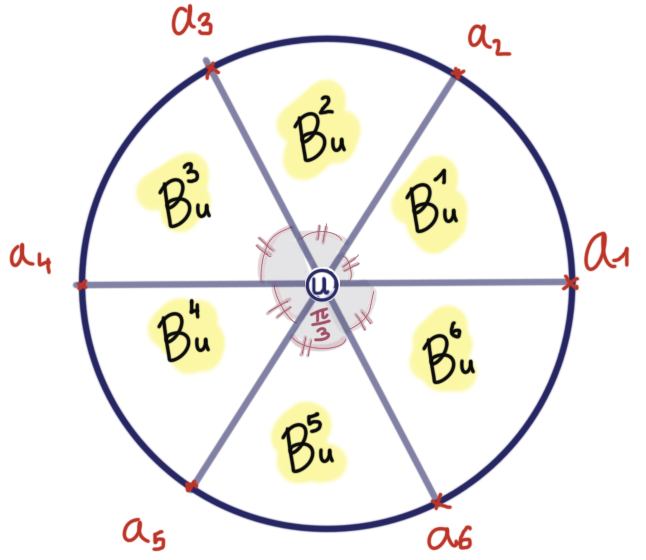}
    \caption{brouillon def des secteurs}
    \label{fig:def-sector}
\end{figure}
At each phase, awake robots focuses only on the $i$-th sector of their ball. The value of $i$ is global : each robot compute $i$ from current time. Selections are done within $i$-th sectors using the closest selection rule.

\subsubsection{Wake up tree computation in \texorpdfstring{$B_u$}{B\_u}}
For each sector $B_u^i$, $u$ computes a wake-up tree \Tree for the selected robots. Given a set of robots contained within a cone, a wake-up tree of bounded makespan $T$ can be computed using strategy from \cite{BCGH24}
%$$T := 1 + \varphi \frac{\pi}{3} \approx 2.7$$

\subsubsection{Propagation}
The awakening of $B_u^i$ is executed by the robots in $B_u^i$ following \Tree.
This implies that when a robot $v$ is awakened by $u$, the first moves of $v$ are dedicated to awakening $B_u^i$. Once it is done $v$ goes back to its initial position and wait until the current phase ends.
At the next phase every awake robots wakes up its $(i+1)$-th sector in particular, $u$ wakes up $B_u^{i+1}$ and $v$ wakes up $B_v^{i+1}$.


\subsection{Upper Bound [Taïssir]}\label{subsection:UDG-upper-bound}

\paragraph{Data structure.}

Each node $u$ stores its initial position \pos and a wake-up tree \wut.
\Taissir{La valeur T est une primitive de l'algo et fait référence à la durée d'une phase.}

\begin{algorithm}[H] \label{algo:UDG}
\caption{UDG Awakening - Code for $u$}
    \Input{$\wut_p$ \text{given by parent if any}}
    %\Output{}
    $I := root(\wut_{\pos})$\tcc*{\Taissir{C'est quoi $I$ ???}}
    $\propagatewut(\wut_p)$\; 
    $\wait(T - (\time() \mod T))$ \tcc*{waits for next phase}
    % For -> "Répéter 6 fois"
    \For(\tcc*[f]{For each sector}){$s \in [1, 6]$}{
    % \Repeat{$6$ times}{
        $i \gets \lceil \time() / T \rceil \mod 6$ \tcc*{sync sector index}
        $p,S, A \gets \snap()$\;
     %   ${\sf cone} \leftarrow S \cap B_u^i$\;
        $\cone \gets \select(p, S \cap B_p^i, A)$\;\nllabel{alg-line:udg-select}
        $\wut \leftarrow \sectorwakeup(p, \cone)$\;
        $\propagatewut(\wut)$\;
        $\move(p)$ \tcc*{Return to initial position}
        $\wait(T - (\time() \mod T))$ \tcc*{waits for next phase}
    }
\end{algorithm}

\paragraph{UDG makespan.}

\begin{theorem}
makespan = O(\ecc) with $O(1)$ energy per node.
\end{theorem}

\begin{proof}
The awakening is divided in phases of fixed duration $T$. We show that $T$ is in $O(1)$ and that the number of phases required to wake up in a UDG is in $O(\ecc)$.

At the beginning of each phase $p$ each awake robot $u$ selects a subset $X_u$ of sleeping robot in its neighbourhood. This subset is such that $X_u \subseteq B^i_{u}$ where $i =(p \mod 6)$ is computed by $u$ thanks to its clock. Since robots shares an absolute coordinate system and a clock, $i$-th sectors of each robot have the same orientation. Lemma~\ref{lem:conflit} states that each robot $u \in \Awake$ can select a set $X_u \subseteq B^i_{u}$ such that $\bigcup_{u \in \Awake} B^i_{u} = \bigcup_{u \in \Awake} X_u$ and for each pair of robots $u, v \in \Awake$, $X_{u} \cap X_{v} = \varnothing$. It implies that each robot $u \in \Awake$ can apply a centralized algorithm on $X_u$ for awakening in parallel $\bigcup_{u \in \Awake} X_u$. From Lemma~\ref{lem:constant-T} with a result for centralized awakening, we can set $T$ the duration of a phase to be a constant, e.g. $2.7$. Finally Lemma~\ref{lem:udg-distance} states that any robot at distance $\ell$ from $s$ is waked up within $12\ell$ phases. As $\ell$ is bounded by \ecc, it follows that Algorithm~\ref{algo:UDG} has a makespan at most $(12\cdot 2.7)\ecc = O(\ecc)$
\end{proof}

\begin{lemma}%\label{lem:constant-T}
    Let $u$ be an awake robot and $X_u$ a set of sleeping robots located in $B^i_u$ for $i \in [1, 6]$. The makespan $T$ for awakening $X_u$ starting from $u$ is at most $2.7$.
\end{lemma}
\begin{proof}
    \cite{BCGH24} gave a strategy to wake up robots located in a sector with a makespan at most $r(1 + \varphi w)$ where $\varphi$ is the golden ratio, $w$ and $r$ are respectively the angle and the length of radii defining the sector. A sector $B^i_u$ has radii of length $1$ and angle $\frac{\pi}{3}$, hence $T \leq 1 + \varphi \frac{\pi}{3} < 2.7$
\end{proof}

\begin{lemma}%\label{lem:udg-distance}
    For any $\ell \in [0, \lceil \ecc \rceil]$ it takes at most $12 \ell$ phase to wake up every robots at distance at most $\ell$ from $s$.
\end{lemma}
\begin{proof}
    Let $\rob_k$ be a robot at distance $\ell$ from $s$ and $\mathcal{P} = (s, \rob_1, ..., \rob_k)$ be a shortest path from $s$ to $\rob_k$ minimizing $k$, the number of edges.
    We show that (1) It takes at most $6k$ phases to wake $\rob_k$ up and (2) The number of edges in $\mathcal{P}$, is upper bounded by $2 \ell$.
    
    \begin{enumerate}
        \item We show by induction that any robot $\rob_i \in \mathcal{P}$ with $0 \leq i \leq k$ is awakened after $6i$ phases at the latest. The base case $s$ is trivial. Assume that $\rob_i$ woke up during the $6i$-th phase. It must have started to awake robots in $B_{\rob_i}$ during the next phase. Any robot in $B_{\rob_i}$ is awakened at most $6$ phases later when each sector of $B_{\rob_i}$ were processed. In particular, either $\rob_{i+1}$ was awoken by $\rob_i$ since there is an edge between $\rob_i$ and $\rob_{i+1}$, $\rob_{i+1} \in B_{\rob_i}$, or it was already awakened. Hence $\rob_{i+1}$ is awakened at most during phase $6{i+1}$.
        \item Let $\rob_j, \rob_{j+1}, \rob_{j+2}$ be three consecutive vertices along $\mathcal{P}$ with $0 \leq j < k-1$. Since $\mathcal{P}$ is a path that minimize the number of edges in a unit disk graph, the distance between two non-consecutive vertices $\rob_j, \rob_{j+2}$ is greater than $1$. If it is not the case, there is an edge between $\rob_{j+1}$ and $\rob_{j+2}$ so $\mathcal{P}$ does not minimize the number of edges since one can replace the two edges $(\rob_{j}, \rob_{j+1})$ and $(\rob_{j+1}, \rob_{j+2})$ by one edge $(\rob_{j}, \rob_{j+2})$.
        Each portion of two consecutive edges along $\mathcal{P}$ has length grater than $1$, and there is exactly $\lfloor \frac{k}{2} \rfloor$ portions of two edges in a path of $k$ edges.
    \end{enumerate}
    Any robot $\rob_k$ is awakened at most at phase $6k$ with $k\leq 2 \ell$ hence any robot $\rob_k$ at distance $\ell$ from $s$ is awakened within at most $12\ell$ phases.
\end{proof}

\begin{lemma}[Conflict]
Let $u$ and $v$ be two awake robots. For any $i \in [1, 6]$ if $B^i_u$ and $B^i_v$ intersects then $|uv| \leq 1$
\end{lemma}%\label{lem:conflit}

\begin{proof}
If there is a robot that is both in the $i$-th sector of $u$ and of $v$ then the radii delimiting the sectors intersects in a  point $w$ such that $|uw| \leq 1$, $|vw| \leq 1$ and $\widehat{uwv} = \frac{\pi}{3}$.
Let $\alpha$ be the widest angle between $\widehat{vuw}$ and $\widehat{wvu}$. One of $\widehat{vuw}$ or $\widehat{wvu}$ must be at least of $\frac{\pi}{3}$ as the sum of angles of the triangle $uvw$ equals $\pi$ so $\alpha \geq \frac{\pi}{3}$ and $\alpha = \max (\widehat{uwv}, \widehat{wvu}, \widehat{vuw})$.
Note that in a triangle the widest angle faces the largest side of the triangle. As $\alpha$ is either the angle that faces $[wv]$ or $[wu]$, the largest side is one of them. Both of $[wv]$ and $[wu]$ are a segment of a radii of length $1$ so their length are at most $1$ by definition. Hence $|uv| \leq \max (|wv|, |wu|) \leq 1$.


\begin{figure}[htbp!]
    \centering
    \includegraphics[width=0.7\linewidth]{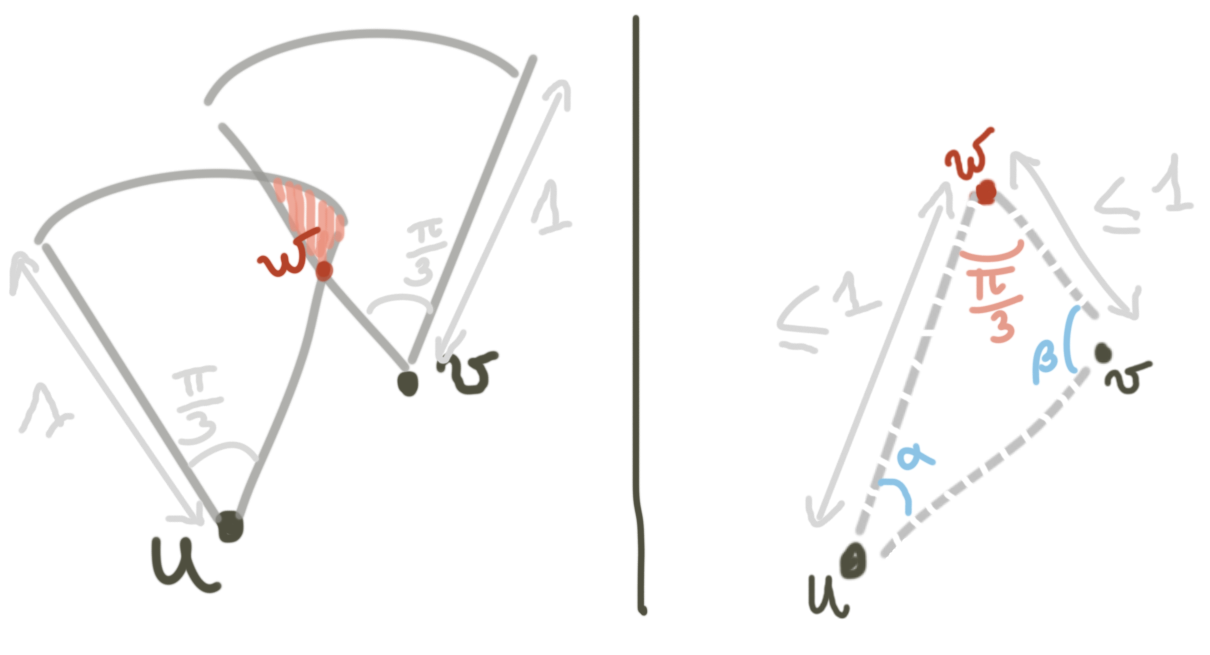}
    \caption{brouillon lemme conflits}
\end{figure}
\end{proof}

\subsection{Lower Bound [Nicolas]}

\begin{theorem}
    For any admissible tuple $(n,1,R)$, there is a point set $\P$ whose unit disk graph $G$ is connected and of eccentricity less than $R^2$ (A PRECISER) such that  any algorithm with $c=O(1)$ energy per robot, the wake-up time is $\Omega(\ecc (G))$.
\end{theorem}

\begin{proof}
    We shall define a point set $\P$ of connectivity threshold $\ell$  with a prescribed eccentricity such that $n\ell \geq \ecc \geq \rho$. Points of $\P=\{p_i\}_{i \leq n}$ are located on a splitted line $A_0,B_0,B_1,A_1,A_2\ldots,A_j,B_j,B_{j+1},A_{j+1},\ldots$ defined by the points $A_j=(0,j(B+1))$ and $B_j=(R/\sqrt{2},j(B+1))$ for even $j \in [0,\ceil{\sqrt{2}\ecc /\rho}{}]$. $s=p_0=A_0$ and $p_1=(\ell,0)$. The other points of $\P$ are spread on the splitted line such that (1) two consecutive points $p_i$ and $p_{i+1}$ are at distance less or equal to $\ell$ from each other and (2) there is at most one point of $\P$ at distance strictly less than $\ell$ per geometric point $A_j$ or $B_j$. The second condition guarantees that $\sum_{i=0}^{n-1} |p_ip_{i+1}|=\ecc$. 
    
    If $B<\ell$, the energy budget is not enough to wake up $\rob_1$ from $\rob_0$. Now assume that $B \geq \ell$. Any wake-up strategy can not be quicker than the eccentricity of $s$ in the $B$-grid graph defined on $\P$. It is impossible to wake up any robot located within a segment $[A_{j+1},B_{j+1}]$ from a robot initially located in $[A_j,B_j]$ because the distance between the two segments is $B+1$. To reach $p_n$, any shortest path within the $B$-grid graph needs to follow a path of length longer than the sum of $|A_jB_j|$, that is at least  $\frac{\rho}{\sqrt{2}}\floor{\sqrt{2}\ecc /\rho}{} \geq \ecc-\frac{\rho}{\sqrt{2}} \geq \ecc(1-1/\sqrt{2}) \geq \ecc/4$.
\end{proof}


\section{Without energy constraint \texorpdfstring{$\ell$}{\ell}-Disk Graph}

\subsection{und [Taïssir]}

\subsubsection{Discovering Functions [Commencé par Gabriel]}

\paragraph{Some Definitions.}

Given two positions $p=(x,y)$ and $p'=(x',y')$, we say that $p$ precedes $p'$, denoted $p\preceq p'$, if $x\leq x'$ and $y\leq y'$.
Given two positions $p\preceq p'$, we call Rectangle between $p$ and $p'$, and denote $\rect(p,p')$ the set of points $\tilde p$ such that $p \preceq \tilde p \preceq p'$.

\paragraph{Main Theorems.}

\begin{theorem}
    There exists a function $DiscoverSolo(p_0,p_f)$ such that when executed at time $t$ by a robot $\rob$ located in $p_0$:
    \begin{itemize}
        \item the function terminates in a time at most $t_f = t_0 + \frac{XY}{\sqrt 3} + X + Y + 2$, where $X = x_f-x_0$ and $Y = y_f - y_0$,
        \item $\rob$ is located at $p_f$ at time $t_f$, and
        \item $\rob$ has discovered all the robots belonging to $\Sleeping(t_f) \cap \rect(p_0,p_f)$.
    \end{itemize}
\end{theorem}
% We present here only the scheme of the algorithm, which will be put into the appendices, as well as the proofs, depending on how long the rest is.
The algorithm we propose simply make the robot travel along the centers of a grid contained in the rectangle, with a vertical increase of $1$ and a horizontal increase of $\sqrt 3$.
Any snapshot includes the rectangle with length $\sqrt 3$ and height $1$, which guarantees that this process indeed covers the entire rectangle.
The number of move necessary to complete this procedure is the number of such elementary rectangles in the complete rectangle, which is less than $\frac{XY}{\sqrt 3} + X + Y + 1$.
\Gabriel{Oui y'a un petit écart entre la complexité annoncée et l'objectif, à voir comment on peut régler ça sans alourdir trop.}

\begin{theorem}
    There exists a function $DiscoverMany(p_0,p_f)$ such that when executed at time $t$ by a robots $\{\rob_1, \dots, \rob_k\}$ colocated in $p_0$:
    \begin{itemize}
        \item the function terminates in a time at most $t_f = t_0 + \frac{XY}{k\sqrt 3} + X + Y + 2$, where $X = x_f-x_0$ and $Y = y_f - y_0$,
        \item $\forall i, \rob_i$ is located at $p_f$ at time $t_f$, and
        \item $\forall i, \rob_i$ has discovered all the robots belonging to $\Sleeping(t_f) \cap \rect(p_0,p_f)$.
    \end{itemize}
\end{theorem}
The general idea is to divide the rectangle into strips of width $X/k$, and to apply the previous algorithm such that each robot discovers one of those strips.


\subsubsection{$\ell$ in a square}
\begin{theorem}
    \label{th:square-L}
    We consider $(\P, \ell)$ a solvable instance.
    Let $\squarereg$ be a square and $P$ be the set of points of its perimeter, such that if $s \in \squarereg$ then $s\in P$.
    We denote by $\squarereg^\square$ the points of $S$ whose distance to $P$ is at most $\ell^2$.
    Let $\P^\square$ be the set of points of $\P \cap \squarereg^\square$ that are connected to $P$ by a path contained in $\squarereg^\square$.
    
    If $|\P^\square| < \ell$, then $\P^\square = \P\cap \squarereg$.
\end{theorem}
\begin{proof}
    Note first that $\P^\square \subset \P\cap \squarereg$.
    Let us therefore consider $u \in \P \cap \squarereg$ and prove that $u\in \P^\square$.
    Since $s \notin \squarereg\setminus P$, $u$ is $\ell$-connected to a point of $P$ (which may be $s$).
    Let us consider a path in the $\ell$-disk graph $v_1v_2\dots v_k=u$, such that $v_1$ is at distance at most $\ell$ from $P$.
    By induction, it appears that $\forall i\in[1,k], v_i$ is at distance at most $i\ell$ from $P$, which means that the first $\ell$ positions on this path are in $\squarereg^\square$, and so, by definition, are in $\P^\square$.
    But since $|\P^\square| < \ell$, we necessarily have $k<\ell$, and thus the entire path belongs to $\P^\square$, which concludes the proof.
\end{proof}

\begin{figure}
    \centering
    \begin{tikzpicture}
        \coordinate (so-big) at (0,0) ;
        \coordinate (se-big) at (5,0) ;
        \coordinate (ne-big) at (5,5) ;
        \coordinate (no-big) at (0,5) ;
        \draw (so-big) -- (se-big) -- (ne-big) -- (no-big) -- (so-big);
        \coordinate (so-smal) at (1,1) ;
        \coordinate (se-smal) at (4,1) ;
        \coordinate (ne-smal) at (4,4) ;
        \coordinate (no-smal) at (1,4) ;
        \draw (so-smal) -- (se-smal) -- (ne-smal) -- (no-smal) -- (so-smal);
        
        \node (inner) at (4.4,4.0) {$\squarereg^{\square}$};
        \coordinate (perim-big) at (2,5);
        \coordinate (perim-smal) at (2,4);
        \draw[->, >=latex] (perim-big) -- (perim-smal) node[right, midway] {$\ell^2$};
    \end{tikzpicture}
    \caption{Scheme of the construction of Theorem~\ref{th:square-L}}
    \label{fig:square-L}
\end{figure}



\subsubsection{Opt DFS}

\begin{algorithm}[H]
\caption{\textsc{DFS - optimisé} - code for $\rob_i$}
\Input{$k$} % à son réveil, le robot "apprend" l'information partagée par les robots réveillés
$\teamsize, \stack, \discovered \gets \share()$\tcc*{Learns current config from other robots}
\If(\tcc*[f]{$B_{p}(\ell)$ is not fully discovered yet}){$B_{p}(\ell) \not\subseteq \discovered$}{
    %$$\;
    $\select, K \gets \textsc{TeamDiscover}(B_p(2\ell), \teamsize$\tcc*[f]{Discover $2\ell$ around $p$}
    $\discovered \gets \discovered + K$\tcc*{Update known environment}
    $\stack.\push(\select)$\tcc*{Stack positions to explore}
}
\While(\tcc*[f]{Repeat until enough robot are awake or until exploration ends}){$\teamsize < k$ \KwAnd \xspace \stack \xspace \KwNot $null$}{
    $\teamsize \leftarrow \teamsize + 1$\;
    $\nxt \leftarrow \stack.\pop()$\;
    $\move(\nxt)$\;
    $\wakeup(\nxt)$\; %départ de DFS 
    %$\share(\teamsize, k, \stack)$\; % en réalité, seul nxt apprend
    \If{$B_{\nxt}(\ell) \not\subseteq K_i$}{
        \stack.\push(\textsc{TeamDiscover}($B_{\nxt}(2\ell), \teamsize$))\;
    }
}
\end{algorithm}

\paragraph{Makespan.}

%$O(\ell^2 \log \min(n, \frac{R}{\ell}) + n\ell)$. 
For any execution of the algorithm, the wake up time of a robot $\rob_i$ is denoted $t_i$ and let $U = \{\rob_i | B_{\rob_i}(\ell) \not\subseteq K_i(t_i)\}$ be the set of robots whose awakening triggered an exploration at distance $2\ell$. 
$$T \leq \sum^{|U|}_{i = 1} \frac{4\ell^2}{i} = O(\ell^2 \log |U|)$$
A robot $\rob \in U$ is at distance greater than $\ell$ from any other robot included in $U$. On the other hand any robot $\rob' \not\in U$ is at distance at most $\ell$ from at least one a robot in included $U$. If it not the case $B_{\rob'}(\ell)$ is not completely explored when $\rob'$ wakes up so it should trigger an exploration of $B_{\rob'}(2\ell)$ and thus $\rob'$ would have been included in $U$ which contradict the assumption that $\rob' \not\in U$.
Thus if $\bigcup_{\rob \in U} B_{\rob}(2\ell)$ is explored it implies the entire surface spanned by the $\ell$-disk graph is explored and $|U| \leq \frac{\rho^2}{\ell^2}$. 
Note that $|U| \leq n$ and $ \frac{\rho}{\ell} \leq \frac{\rho^2}{\ell^2}$ ; the upper bound follows.

\subsubsection{Separator}



\paragraph{Description haut niveau.}

Let \squarereg be a square region of the plane centered in the source robot $s$, with side length $R = 2 \rho(\P, s)$ and such that $\P \subseteq \squarereg$.
The Separator algorithm relies on a Divide-and-conquer technique thus the goal is to recursively split \squarereg into separated regions of decreasing size. At each iteration, we alternate between exploration \Taissir{"Separating exploration" ?} and recruitment. Both step are required in order to verify some pre-condition before recursively awakening each sub region.


\begin{enumerate}
    \item \textbf{Initialization:} Starting from the center of $\squarereg$ we form a team \team of $\ell$ robots in time $O(\ell + \ell^2 \log \ell)$. (using DFS opt)
    \item \label{item:begin-separator} If $|\team| < \ell$, from Theorem~\ref{th:square-L} there is no robot left asleep in \squarereg and the algorithm stops. From here, we assume there are $\ell$ robots located at the center of \squarereg
    \begin{enumerate}
        \item \textbf{(Base case)} If \squarereg has side of length $R \leq \ell^{\frac{3}{2}}$, explore \squarereg with \team in $O(\ell^2)$, compute a wake-up tree with a centralized algorithm and wake up everyone in $O(\ell^{\frac{3}{2}})$.
        \item The region \squarereg is partitioned into four squares $\squarereg[1], \squarereg[2], \squarereg[3], \squarereg[4]$. The team split into 4 teams $\team_1, \team_2, \team_3, \team_4$. For $i \in [1, 4]$, in parallel, $\team_i$ explore and recruit in $\squarereg[i]$:
        \begin{itemize}
            \item $\team_i$ follows the perimeter of $\squarereg[i]$ to sweep a Separator area of width $\ell$ in $O(R)$ time.
            \item $\team_i$ recruit $\ell$ robots from \squarereg[i] in $O(R+\ell^2)$ time
            \item Go back to the center of \squarereg.
        \end{itemize}
    \item The team \team reunite and shares everything.
    \item Each awake robot $\rob_j$ move to the center of the square $\squarereg[i]$ such that $p_j \in \squarereg[i]$.
    \item (repeat the process from step~\ref{item:begin-separator})
    \end{enumerate}
\end{enumerate}

\paragraph{Recruitment.} A robot is \emph{native} to a region \squarereg[i] if its initiate position is contained in \squarereg[i]. The goal of the recruitment in a sub-square \squarereg[i] is to pick up $4\ell$ awake robots native to \squarereg[i] to constitute a team denoted $\team(\squarereg[i])$. This prepare the recursive step where each square \squarereg[i] is taken over by the team $\team(\squarereg[i])$ thus recruited: Since every robot goes back to its initial square region before waking-up recursively the sub-squares, any robot native to \squarereg[i] is part of $\team(\squarereg[i])$ even if it is currently absent from the region \squarereg[i]. A recruited robot is either a robot awakened on the fly during the recruitment phase or a robot previously waked-up in \squarereg[i].

Let $\team_i$ be a team of $\ell$ robots affected to $\squarereg[i]$ and $\X_i$ be the set of initial positions in the Separator $\squarereg[i]^{\square}$: $\X_i = \{\pos[j] | \pos[j] \in \squarereg[i]^{\square}\}$. For each $\pos[j] \in \X_i$ let $x_j$ be the orthogonal projection of $\pos[j]$ onto the nearest side of \squarereg[i] (i.e. a segment of the perimeter). If needed, break ties arbitrarily. The recruitment path consist of $\team_i$ travelling along the perimeter of \squarereg[i] until it reaches a projection $x_j$. When it is the case, $\team_i$ move to $\pos[j]$ which is at most at distance $\ell$ from $x_j$. From there and for every other position $\pos[j] \in X_i$, $\team_i$ starts a DFS from $\pos[j]$ until either it reaches the end of a branch of $|\team(\squarereg[i])| \geq 4\ell$.


\begin{theorem}
    \label{th:separator-old}
    \Taissir{C'est le théorème \ref{th:upper} en fait.}
    We consider $(\P, s)$ an admissible instance with radius $\rho$. The separator algorithm achieve awakening within $O(\rho + \ell^2 \log \frac{\rho^2}{\ell^{\frac{3}{2}}})$ time.
\end{theorem}

\begin{proof}

\begin{itemize}
    \item The number of recursive step is at most $\log_2(\frac{R^2}{\ell^{\frac{3}{2}}})$
\end{itemize}
\end{proof}


\begin{lemma}
    \Taissir{Conséquence du théorème~\ref{th:square-L} ??}
    The set of positions contained in a perimeter \Taissir{Definition de Séparateurs pour éviter confusion avec périmètre} of width $\ell$ is a separating set in the $\ell$-disk graph.
\end{lemma}
Since the last task of $\team_i$ was the exploration of the Separator, either $X_i$ contains at least one position or the full square \squarereg[i] is empty. If a robot $\rob_k$ is initially located in the interior of the square, $\pos[k] \in \squarereg[i] \backslash \squarereg[i]^{\square}$ then there must be a path from a position of $\pos[j] \in \X_i$ to $\pos[k]$ in the $\ell$-disk graph. Hence any robot in \squarereg[i] can be reached with a depth-first search in the $\ell$-disk graph rooted in $p_j$. It follows that if $|\X_i| = 0$ then the interior of $\squarereg[i]$ is empty (this is because $\X_i$ is a separator in the $\ell$-disk graph). 
Our strategy for recruiting robots in $\squarereg[i]$ is based on this property: while it is possible and until $|\team(\squarereg[i])| = 4\ell$, explore \squarereg[i] along a path of the $\ell$-disk graph starting from the positions in $\X_i$.

\begin{lemma}
    A recursive step lasts at most $O(R + \ell^2)$ time.
    (1) Exploring the separators in time $O(R)$ (2) The recruitment takes at most $O(R + \ell^2)$
\end{lemma}
\begin{proof}
During each step and for each sub-squares \squarereg[i], two main tasks are performed by a team $\team_i$ of $O(\ell)$ robots: separating \squarereg[i] by exploring its perimeter \Taissir{périmètre vs séparateur} and recruiting $\ell$ robots in $\squarereg[i]$. 
The area of $\squarereg[i]^{\square}$ is $O(R\ell)$ and the exploration is distributed among the $O(\ell)$ robots of $\team_i$ so each of them cover a path of length $O(R)$.
The duration of the recruitment is made of the sum of the length of each branch of the depth-first search rooted in a position in $\X_i$ and the sum of the distance between two start position of $\X_i$.
En décomposant le trajet effectué :
\begin{itemize}
    \item The length of the monotonic path is at most $O(R + \ell^2)$:
    \item The sum of each DFS branch is $O(\ell^2)$ : 
\end{itemize}
    
    
\end{proof}



%\paragraph{Explicit construction.}
%Given an execution of algorithm $\A$ with inputs $n,R,\ell$ on the plane with set of robots $\P$,
%we denote by $D_\P(t)$ the set of discovered points at time $t$, which are the points $p$ such that $\exists t' \leq t, \exists r\in \Awake(t'): |p_r(t')p| \leq 1$.
%Finally, we denote by $E_\P(t)$ the area of $D_\P(t)$.

%For any $c \in \centers_m$, we define $t_c(\P) = \inf \{t \geq 0 \mid S_c \subseteq D_\P(t) \}$, and for any $c \in \centers_m$, let $p_c(\P)$ be a point of $S_c$ such that $\forall t<t_c(\P), p_c(\P) \notin D_\P(t)$.
%Note that the definition of $p_c(\P)$ remains valid if $t_c(\P) = +\infty$.
%Note that by Lemma~\ref{lem:all-discovered}, we can suppose that all $t_c$ are finite.


% \begin{lemma}
%     \label{lem:time-to-explore}
%     Let $t' < t$, we have $E(t)-E(t') \leq 2(t-t') \times |\Awake(t)|$.
% \end{lemma}

% \begin{lemma}
%     \label{lem:all-discovered}
%     If $\exists S_c \in \spheres: t_c = +\infty$ then algorithm $\A$ does not solve $FT$.
% \end{lemma}
